# Supplementary material for: CorBenchX: Large-Scale Chest X-Ray Error Dataset and Vision-Language Model Benchmark for Report Error Correction
Source: arXiv:2505.12057 source file (2025-05-17)
Supplement: Supplementary file 1 [file Appendix.tex]

\newpage
\appendix

\section{Technical Appendices and Supplementary Material}

licenses of public datasets

prompt

hyper parameters
